# Supplementary material for: Video DataFlywheel: Resolving the Impossible Data Trinity in Video-Language Understanding
Source: arXiv:2409.19532 source file (2024-09-29)
Supplement: Supplementary file 1 [file exp_setting.tex]

\section{Experiment Setting} \label{sec:sup_exp_setting}

More details on image SFT dataset.

More details on GPT-3.5 evaluation.

Optimal hyper-parameters of noise control baselines.
